# Supplementary material for: Interacting Weyl fermions: Phases, phase transitions and global phase diagram
Source: arXiv:1610.05762 ancillary file (2017-05-05)
Supplement: Supplementary file 1 [file WeylCriticality_Supplementary.pdf]

# Supplementary Materials for “Interacting Weyl fermions: Phases, phase transitions and global phase diagram”

Bitan Roy,<sup>1,2</sup> Pallab Goswami,<sup>1</sup> and Vladimir Juričić<sup>3</sup>

<sup>1</sup>*Condensed Matter Theory Center and Joint Quantum Institute, Department of Physics, University of Maryland, College Park, Maryland 20742- 4111 USA*

<sup>2</sup>*Department of Physics and Astronomy, Rice University, Houston, Texas 77005, USA*

<sup>3</sup>*Nordita, Center for Quantum Materials, KTH Royal Institute of Technology and Stockholm University, Roslagstullsbacken 23, 10691 Stockholm, Sweden*

In the present Supplementary Materials we address the followings.

1. Derivation of the continuum (low-energy) Hamiltonian for Weyl systems from a tight-binding lattice model,
2. Computation of monopole charge of general Weyl semimetal (WSM) from low-energy description,
3. Fierz constraint among four-fermion interactions among two and four component fermions in Weyl systems,
4. Renormalization (RG) analysis inside the WSM in the presence of generic local interactions,
5. RG flow of various source terms in a WSM in the presence of generic local interactions,
6. Solution of the gap equation in axionic insulator phase in a general WSM,
7. Derivation of free-energy at the Weyl semimetal-insulator quantum critical point in the presence of short-range interaction.

## I. LATTICE MODEL FOR WEYL SYSTEMS

As mentioned in the main part of the paper, all types of Weyl semimetals (WSMs) can be realized from a simple two-band model  $H = \sum_{\mathbf{k}} \psi_{\mathbf{k}}^\dagger [\mathbf{N}(\mathbf{k}) \cdot \boldsymbol{\sigma}] \psi_{\mathbf{k}}$ , after suitably choosing the spin/pseudospin vector  $\mathbf{N}(\mathbf{k})$ , where  $\psi_{\mathbf{k}}^\top = (c_{\mathbf{k},\uparrow}, c_{\mathbf{k},\downarrow})$  is a two component spinor,  $c_{\mathbf{k},\alpha}$  is the fermion annihilation operator with momentum  $\mathbf{k}$  and (pseudo)spin projection  $\alpha = \uparrow, \downarrow$ , and  $\boldsymbol{\sigma}$  are Pauli matrices. We here demonstrate how to arrive at the continuum model [see Eq. (1) of main text] for Weyl systems starting from a tight-binding model for  $n = 1$  (simple WSM). Our construction can then easily be generalized to find the correspondence between lattice and continuum models for  $n = 2$  and  $3$  (general WSM). A simple WSM can be realized by choosing

$$N_1(\mathbf{k}) = t \sin k_x, N_2(\mathbf{k}) = t \sin k_y, N_3(\mathbf{k}) = [t_z \cos(k_z a) - m_z] + t_0 [2 - \cos(k_x a) - \cos(k_y a)]. \quad (1)$$

With the above choice of pseudospin vector the Weyl nodes are located at  $\mathbf{k} = (0, 0, \pm k_z^0)$ , where

$$\cos(k_z^0 a) = \frac{t_0}{t_z} \left[ \frac{m_z}{t_0} + \cos(k_x a) + \cos(k_y a) - 2 \right]. \quad (2)$$

Finally expanding the above Hamiltonian  $H$  around the  $\Gamma = (0, 0, 0)$  point of the Brillouin zone we arrive at the following continuum model

$$\hat{H}_{n=1}(\Delta) = v (\sigma_1 k_x + \sigma_2 k_y) + \sigma_3 (B k_z^2 + \Delta), \quad (3)$$

where  $v = ta$  is the Fermi velocity in the  $xy$  plane and  $B = t_z a^2/2$  bears the dimension of inverse mass, and  $\Delta = m_z - t_z$ . The above Hamiltonian assumes the form of  $H_n$  from Eq. (1) of the main text for  $n = 1$ , with  $\alpha_1 = v$ . In the final expression we have omitted a term proportional to  $\sigma_3 k_z^2$ , as this term is an irrelevant quantity under coarse graining. For  $\Delta < 0$ , further linearizing the above Hamiltonian about  $\pm \mathbf{K}_z$ , where  $\mathbf{K}_z = \sqrt{-\Delta/B}$ , we arrive at the familiar Hamiltonian for simple WSM with  $n = 1$

$$H_{n=1} = v (\tau_0 \sigma_1 k_x + \tau_0 \sigma_2 k_y) + v_z \tau_3 \sigma_3 k_z. \quad (4)$$

In the last equation  $k_z$  is measured from  $\pm \mathbf{K}_z$ , with  $v_z = 2B\sqrt{-\Delta/B}$  bearing the unit of Fermi velocity. The new set of Pauli matrices  $\tau_\mu$  operate on the chiral, namely left and right, indices.

A double WSM can be realized by choosing

$$\begin{aligned} N_1(\mathbf{k}) &= t(\cos k_x - \cos k_y), N_2(\mathbf{k}) = t \sin k_y \sin k_y, \\ N_3(\mathbf{k}) &= [t_z \cos(k_z a) - m_z] + t_0 \{[3 + \cos 2k_x - 4 \cos k_x] + [3 + \cos 2k_y - 4 \cos k_y]\}. \end{aligned} \quad (5)$$

Linearizing the Hamiltonian with such choice of pseudo-spin vectors about  $\Gamma = (0, 0, 0)$  we arrive at the following continuum model

$$\hat{H}_{n=2}(\Delta) = \frac{1}{m} (\sigma_1 [k_x^2 - k_y^2] + \sigma_2 [2k_x k_y]) + \sigma_3 (Bk_z^2 + \Delta), \quad (6)$$

where  $m = -2/(ta^2)$  bears the unit of mass. In the last expression we have neglected terms proportional to  $k_x^4$  and  $k_y^4$  as they are irrelevant in RG sense in comparison to  $k_x^2 - k_y^2$  and  $k_x k_y$ . Finally, linearizing the term proportional to  $\sigma_3$  about  $\pm \mathbf{K}_z$  we arrive at the low energy Hamiltonian for double WSM

$$\hat{H}_{n=2}(\Delta) = \frac{1}{m} (\tau_0 \sigma_1 [k_x^2 - k_y^2] + \tau_0 \sigma_2 [2k_x k_y]) + v_z \tau_3 \sigma_3 k_z, \quad (7)$$

as announced in the main part of the paper.

A triple WSM can be realized with the following choices of the pseudo-spin vectors

$$\begin{aligned} N_1(\mathbf{k}) &= t \sin k_x [(1 - \cos k_x) - 3(1 - \cos k_y)], N_2(\mathbf{k}) = -t \sin k_y [(1 - \cos k_y) - 3(1 - \cos k_x)], \\ N_3(\mathbf{k}) &= [t_z \cos(k_z a) - m_z] + t_0 \{[3 + \cos 2k_x - 4 \cos k_x] + [3 + \cos 2k_y - 4 \cos k_y]\}. \end{aligned} \quad (8)$$

Expanding the tight-binding Hamiltonian around  $\Gamma = (0, 0, 0)$  point of the Brillouin zone we arrive at the following low-energy model

$$\hat{H}_{n=3}(\Delta) = \alpha_3 (\sigma_1 [k_x^3 - 3k_x k_y^2] - \sigma_2 [k_y^3 - 3k_y k_x^2]) + \sigma_3 (Bk_z^2 + \Delta), \quad (9)$$

where  $\alpha_3 = ta^3/2$ . Finally, expanding the term proportional to  $\sigma_3$  about the Weyl nodes at  $\pm \mathbf{K}_z$  we arrive at the low-energy theory for the triple WSM

$$\hat{H}_{n=3}(\Delta) = \alpha_3 (\tau_0 \sigma_1 [k_x^3 - 3k_x k_y^2] - \tau_0 \sigma_2 [k_y^3 - 3k_y k_x^2]) + v_z \tau_3 \sigma_3 k_z, \quad (10)$$

as announced in the main part of the paper.

## II. MONOPOLE CHARGE OF GENERAL WEYL NODES FROM CONTINUUM THEORY

We here present the computation of the monopole charge of Weyl node of general WSM within the continuum description of these system, respectively displayed in Eqs. (4), (7), (10) for single ( $n = 1$ ), double ( $n = 2$ ) and triple ( $n = 3$ ) WSM. For concreteness, we here focus on the monopole (accommodating left chiral fermions), near which the Hamiltonian can compactly be written as

$$H_n^+ = \alpha_n k_\perp^n \cos(n\phi_{\mathbf{k}}) \sigma_1 + \alpha_n k_\perp^n \sin(n\phi_{\mathbf{k}}) \sigma_2 + v_z k_z \sigma_3, \quad (11)$$

for  $n = 1, 2, 3$ . Upon introducing a new set of parameters according to

$$\frac{v_z k_z}{E_{\mathbf{k}}} = \cos \theta_{\mathbf{k}}, \quad \frac{\alpha_n k_\perp^n}{E_{\mathbf{k}}} = \sin \theta_{\mathbf{k}}, \quad (12)$$

with  $0 \leq \theta_{\mathbf{k}} \leq \pi$ ,  $0 \leq \phi_{\mathbf{k}} < 2\pi$ , where  $E_{\mathbf{k}} = \sqrt{v_z^2 k_z^2 + \alpha_n^2 k_\perp^{2n}}$ , the above Hamiltonian can compactly be written as

$$H_n^+ = E_{\mathbf{k}} [\sin \theta_{\mathbf{k}} \cos(n\phi_{\mathbf{k}}) \sigma_1 + \sin \theta_{\mathbf{k}} \sin(n\phi_{\mathbf{k}}) \sigma_2 + \cos \theta_{\mathbf{k}} \sigma_3] \equiv \mathcal{N}_{\mathbf{k}} \cdot \sigma. \quad (13)$$

Here,  $\mathcal{N}_{\mathbf{k}}$  represents the pseudo-spin vector, and the corresponding pseudo-spin unit vector is defined as  $\mathbf{n}_{\mathbf{k}} = \mathcal{N}_{\mathbf{k}}/|\mathcal{N}_{\mathbf{k}}|$ , with

$$\mathbf{n}_{\mathbf{k}} = [\sin \theta_{\mathbf{k}} \cos(n\phi_{\mathbf{k}}), \sin \theta_{\mathbf{k}} \sin(n\phi_{\mathbf{k}}), \cos \theta_{\mathbf{k}}]. \quad (14)$$

The Weyl node that acts as a source (or sink) of Abelian Berry curvature and represents a defect in the momentum space is characterized by the topological invariant

$$W_n = \frac{1}{4\pi} \int_0^{2\pi} d\phi_{\mathbf{k}} \int_0^\pi d\theta_{\mathbf{k}} \left[ \mathbf{n}_{\mathbf{k}} \cdot \left( \frac{\partial \mathbf{n}_{\mathbf{k}}}{\partial \theta_{\mathbf{k}}} \times \frac{\partial \mathbf{n}_{\mathbf{k}}}{\partial \phi_{\mathbf{k}}} \right) \right] = n. \quad (15)$$

Therefore,  $W_n$  characterizes the strength of monopole ( $n$ ) that in turn also defines the integer topological invariant of a general WSM.

### III. FIERZ IDENTITY FOR LOCAL FOUR-FERMION INTERACTIONS

*Two-component fermion:* The interacting Hamiltonian for a two component spinor in the presence of generic short-range interaction reads as

$$H_{int}^1 = \int d^3x \left[ g_0 (\psi^\dagger \sigma_0 \psi)^2 + g_1 (\psi^\dagger \sigma_1 \psi)^2 + g_2 (\psi^\dagger \sigma_2 \psi)^2 + g_3 (\psi^\dagger \sigma_3 \psi)^2 \right], \quad (16)$$

where  $\psi$  is a two-component spinor, describing the critical excitations residing at the quantum critical point (QCP) between the WSM and symmetry preserving band insulator. Here,  $\sigma_j$  for  $j = 1, 2, 3$  are standard Pauli matrices and  $\sigma_0$  is the two-dimensional identity matrix. For generality we set  $g_1 \neq g_2$ , although in Weyl systems  $g_1 = g_2$  (due to in-plane rotational symmetry). However, not all four coupling constant are linearly independent. Existence of Fierz identity, written as

$$[\psi^\dagger(x) \sigma_a \psi(x)] [\psi^\dagger(y) \sigma_b \psi(y)] = -\frac{1}{4} \text{Tr} [\sigma_a \sigma_c \sigma_b \sigma_d] [\psi^\dagger(x) \sigma_c \psi(y)] [\psi^\dagger(y) \sigma_d \psi(x)], \quad (17)$$

where  $a, b, c, d = 0, 1, 2, 3$ , and for local interaction  $x = y$ , allows one to rewrite each quartic interaction as a linear combination of others. To find the number of independent coupling constants we define a four-dimensional vector as

$$X^\top = \left[ (\psi^\dagger \sigma_0 \psi)^2, (\psi^\dagger \sigma_1 \psi)^2, (\psi^\dagger \sigma_2 \psi)^2, (\psi^\dagger \sigma_3 \psi)^2 \right], \quad (18)$$

with the Pauli matrices as a basis in the space of  $2 \times 2$  hermitian matrices. The above Fierz constraint can then be compactly written as  $F_{4 \times 4} X = 0$ , where

$$F_{4 \times 4} = \begin{bmatrix} 3 & 1 & 1 & 1 \\ 1 & 3 & -1 & -1 \\ 1 & -1 & 3 & -1 \\ 1 & -1 & -1 & 3 \end{bmatrix}. \quad (19)$$

The rank of  $F_{4 \times 4}$  is 3 and therefore the number of linearly independent coupling constant is  $4 - 3 = 1$ . We chose  $g_3$  as the independent coupling constant. Then the rest of the coupling constants related to  $g_3$  according to

$$g_0 = -g_3, \quad g_1 = g_3, \quad g_2 = g_3. \quad (20)$$

*Four-component fermion:* Next we turn our focus on the interacting theory for a four-component fermion, which can be realized deep inside the WSM phase. Upon imposing all microscopic and emergent symmetries the interacting Hamiltonian reads as

$$H_{int}^W = \int d^3x \left[ g_0 (\Psi^\dagger \Psi)^2 + \sum_{j=1}^2 \left\{ g_1 \left[ (\Psi^\dagger \gamma_j \Psi)^2 + (\Psi^\dagger \Gamma_{j5} \Psi)^2 \right] + g_2 (\Psi^\dagger \Gamma_{0j} \Psi)^2 + g_3 (\Psi^\dagger \Gamma_{j3} \Psi)^2 \right\} + g_4 \left[ (\Psi^\dagger \gamma_0 \Psi)^2 + (\Psi^\dagger \Gamma_{05} \Psi)^2 \right] + g_5 \left[ (\Psi^\dagger \gamma_3 \Psi)^2 + (\Psi^\dagger \Gamma_{35} \Psi)^2 \right] + g_6 (\Psi^\dagger \gamma_5 \Psi)^2 + g_7 (\Psi^\dagger \Gamma_{03} \Psi)^2 + g_8 (\Psi^\dagger \Gamma_{12} \Psi)^2 \right], \quad (21)$$

where  $\Gamma_{jk} = i\gamma_j \gamma_k$  and  $\Psi$  is now a four-component spinor. However, not all the quartic couplings are linearly independent as they are related to each other by the Fierz relation

$$[\Psi^\dagger(x) M \Psi(x)] [\Psi^\dagger(y) N \Psi(y)] = -\frac{1}{16} \text{Tr} [M \Gamma_a N \Gamma_b] [\Psi^\dagger(x) \Gamma_a \Psi(y)] [\Psi^\dagger(y) \Gamma_b \Psi(x)], \quad (22)$$

which we apply here for contact interaction  $x = y$ . Here  $M$  and  $N$  are  $4 \times 4$  hermitian matrices, and  $\Gamma_a$  close the basis for all  $4 \times 4$  hermitian matrices,  $a, b = 1, \dots, 16$ . To capture the number of independent coupling constants we define a nine component vector

$$X^\top = \left[ (\Psi^\dagger \Psi)^2, (\Psi^\dagger \gamma_1 \Psi)^2 + (\Psi^\dagger \gamma_2 \Psi)^2 + (\Psi^\dagger \gamma_{15} \Psi)^2 + (\Psi^\dagger \gamma_{25} \Psi)^2, (\Psi^\dagger \gamma_{01} \Psi)^2 + (\Psi^\dagger \gamma_{02} \Psi)^2, (\Psi^\dagger \gamma_{13} \Psi)^2 + (\Psi^\dagger \gamma_{23} \Psi)^2, (\Psi^\dagger \gamma_0 \Psi)^2 + (\Psi^\dagger \gamma_{05} \Psi)^2, (\Psi^\dagger \gamma_3 \Psi)^2 + (\Psi^\dagger \gamma_{35} \Psi)^2, (\Psi^\dagger \gamma_5 \Psi)^2, (\Psi^\dagger \gamma_{03} \Psi)^2, (\Psi^\dagger \gamma_{12} \Psi)^2 \right]. \quad (23)$$

The Fierz constraints can be written compactly as  $F_{9 \times 9} X = 0$ , where

$$F_{9 \times 9} = \begin{bmatrix} 5 & 1 & 1 & 1 & 1 & 1 & 1 & 1 & 1 \\ 1 & 1 & 0 & 0 & 0 & 0 & -1 & 1 & -1 \\ 1 & 0 & 2 & 0 & -1 & 1 & 1 & -1 & -1 \\ 1 & 0 & 0 & 2 & 1 & -1 & 1 & -1 & -1 \\ 1 & 0 & -1 & 1 & 2 & 0 & -1 & -1 & 1 \\ 1 & 0 & 1 & -1 & 0 & 2 & -1 & -1 & 1 \\ 1 & -1 & 1 & 1 & -1 & -1 & 5 & 1 & 1 \\ 1 & 1 & -1 & -1 & -1 & -1 & 1 & 5 & 1 \\ 1 & -1 & -1 & -1 & 1 & 1 & 1 & 1 & 5 \end{bmatrix}. \quad (24)$$

The rank of the matrix is 5 and therefore there are five relations among the nine couplings, and the number of independent coupling constants is thus  $9 - 5 = 4$ . We choose  $g_0, g_2, g_3$  and  $g_4$  as independent coupling constants. The remaining quartic terms are related to these four couplings according to

$$g_1 = -4g_0 - 2g_3 - 2g_4, \quad g_5 = -g_2 + g_3 + g_4, \quad g_6 = -g_0 - \frac{g_2}{2} - \frac{g_3}{2}, \quad g_7 = g_0 + g_3 + g_4, \quad g_8 = -g_0 + \frac{g_2}{2} - \frac{g_3}{2} - g_4. \quad (25)$$

#### IV. RENORMALIZATION GROUP ANALYSIS INSIDE THE WEYL SEMIMETAL PHASE

Let us now present details of the RG calculation in a general WSM in the presence of short-range interactions. As mentioned in the main part of the paper the scaling dimension of any short-range interaction is  $[g_j] = -2/n$ . Hence, short-range interaction is marginal ( $[g_j] = 0$ ) as  $n \rightarrow \infty$ , which corresponds to a hypothetical situation where the system effectively behaves as one-dimensional, constituted by linearly dispersing (along  $k_z$ ) chiral fermions and the density of states is finite. Thus our RG calculation can be controlled via a  $1/n$  expansion and  $[g_j] = -\epsilon$ , where  $\epsilon = 2/n$ . The imaginary time ( $\tau$ ) action for general WSM in the presence of short-range interaction reads as

$$S = \int \frac{d\tau d^2x_\perp dz}{(2\pi)^4} \left[ \Psi [\partial_\tau + H_W^n(\mathbf{k} \rightarrow -i\nabla)] \Psi + \sum_j g_j (\Psi^\dagger M_j \Psi)^2 \right], \quad (26)$$

where  $H_W^n(\mathbf{k})$  is the Hamiltonian for general WSM, supporting Weyl nodes of monopole strength  $n$ , summation over  $j$  runs over all four local quartic terms, and  $M_j$ s are corresponding Hermitian matrices. We now integrate out the fast Fourier modes within the shell  $E_c e^{-l} < \sqrt{\omega^2 + v^2 k_z^2} < E_c$  and  $0 < (k_\perp^n \alpha_n / E_c)^{2/n} < \infty$  and subsequently rescale the co-ordinates according to  $\tau \rightarrow e^{-l} \tau$ ,  $(x, y) \rightarrow e^{-l/n} (x, y)$ ,  $z \rightarrow e^{-l} z$  and fermionic field  $\Psi \rightarrow e^{(1+\frac{2}{n})l} \Psi$  to arrive at the following flow equations of various coupling constants to the leading order in  $\epsilon$ -expansion. The relevant shell integrals for one-loop RG calculations are

$$\int \frac{d\omega dk_z}{(2\pi)^2} \frac{d\mathbf{k}_\perp}{(2\pi)^2} \frac{\omega^2}{D^2} = \int \frac{d\omega dk_z}{(2\pi)^2} \frac{d\mathbf{k}_\perp}{(2\pi)^2} \frac{v^2 k_z^2}{D^2} = f_1(n) a_\epsilon l + \mathcal{O}(l^2), \quad \int \frac{d\omega dk_z}{(2\pi)^2} \frac{d\mathbf{k}_\perp}{(2\pi)^2} \frac{\alpha_n^2 k_\perp^{2n}}{D^2} = f_2(n) a_\epsilon l + \mathcal{O}(l^2), \quad (27)$$

where  $D = [\omega^2 + v^2 k_z^2 + \alpha_n^2 k_\perp^{2n}]$ ,  $a_\epsilon = E_c^\epsilon / (32\pi^3 \alpha_n^\epsilon)$  and

$$f_1(n) = \frac{\pi(n-1) \csc(\frac{\pi}{n})}{n^2} = 1 - \frac{1}{n} + \mathcal{O}(n^{-2}), \quad f_2(n) = \frac{\pi \csc(\frac{\pi}{n})}{n^2} = \frac{2}{n} + \mathcal{O}(n^{-2}), \quad (28)$$

Therefore, as  $n \rightarrow \infty$  only the contribution from  $f_1(n)$  survives and  $f_2(n)$  captures subleading divergence, which off course vanishes as  $n \rightarrow \infty$ . After computing the standard one-loop diagrams, we arrive at the following RG flow equations for four-fermion coupling constants

$$\begin{aligned} \beta_{\lambda_0} &= -\epsilon \lambda_0 + \lambda_0 \left\{ \left[ \lambda_2 + \lambda_3 + \lambda_4 - \frac{\lambda_0}{2} \right] + \delta_{n,2p+1} [-\lambda_2 + \lambda_3 - 2\lambda_4] + \delta_{n,2p} [\lambda_2 - \lambda_3] \right\} f_2(n), \\ \beta_{\lambda_2} &= -\epsilon \lambda_2 + \{ \lambda_2^2 - \lambda_3^2 + \lambda_4^2 + \lambda_2(2\lambda_4 - \lambda_0) + \lambda_0(\lambda_3 - \lambda_4) \} f_1(n) + \delta_{n,2p+1} \lambda_2 \left[ \frac{\lambda_0}{2} - \lambda_4 \right] f_2(n) \\ &\quad + \delta_{n,2p} \left[ \frac{\lambda_0^2}{4} + \lambda_2^2 + \lambda_3^2 + \frac{\lambda_4^2}{2} - \lambda_3 \left( \frac{\lambda_0}{2} - \lambda_4 \right) \right] f_2(n), \end{aligned}$$

$$\begin{aligned}
\beta_{\lambda_3} &= -\epsilon\lambda_3 + \{\lambda_3(2\lambda_3 - \lambda_0 - 2\lambda_2 - 2\lambda_4) + \lambda_0(\lambda_2 + \lambda_4)\} f_1(n) + \delta_{n,2p+1} \left\{ \lambda_0 \left[ \lambda_3 - \lambda_4 - \frac{\lambda_2}{2} \right] + \lambda_4 \left[ \lambda_2 + \frac{\lambda_4}{2} \right] \right\} f_2(n) \\
&\quad + \delta_{n,2p}\lambda_3 \left( 2\lambda_2 + \lambda_4 - \frac{\lambda_0}{2} \right) f_2(n), \\
\beta_{\lambda_4} &= -\epsilon\lambda_4 + [2\lambda_4^2 + \lambda_4(-\lambda_0 + 2\lambda_2 - 2\lambda_3)] \left[ f_1(n) + \frac{f_2(n)}{2} \right] + [\lambda_2^2 + \lambda_3^2 - \lambda_4^2 + \lambda_0\lambda_4 - 2\lambda_2\lambda_3] f_1(n) \\
&\quad + \{\delta_{n,2p+1} [\lambda_0(\lambda_3 - \lambda_2 - \lambda_4) + \lambda_4(\lambda_2 + \lambda_3)] + \delta_{n,2p}\lambda_4(\lambda_2 + \lambda_3)\} f_2(n)
\end{aligned} \tag{29}$$

to the leading order in  $\epsilon$ -expansion, where  $\delta$  is the Kronecker delta function,  $p$  is an integer, and  $\lambda_j = g_j E_c^\epsilon / (4\pi^3 \alpha_n^\epsilon)$  are dimensionless coupling constants for  $j = 0, 2, 3, 4$ . The distinction between the RG flow equations for a WSM with an even and odd monopole charge arises from the fact that the free propagator is an odd function of the momentum in the latter case, while it is an even function of the in-plane component of momentum ( $k_x, k_y$ ) and odd function of  $k_z$  in the former case. The flow equations to the leading order in  $1/n$  have already been reported in the main part of the paper, which altogether support three fixed points.

Upon incorporating  $1/n$  corrections, the RG flow equations still support three fixed points. The fully stable non-interacting Gaussian fixed point is located at  $(\lambda_0, \lambda_2, \lambda_3, \lambda_4) = (0, 0, 0, 0)$ . Two QCPs are now located at

$$\begin{aligned}
(a) &\approx \left( 0, -\frac{1}{4} + \frac{0.3}{n}\delta_{n,2p} + \frac{0.06}{n}\delta_{n,2p+1}, \frac{1}{2} + \frac{0.15}{n}\delta_{n,2p} + \frac{0.06}{n}\delta_{n,2p+1}, \frac{1}{4} - \frac{0.11}{n}\delta_{n,2p} - \frac{0.06}{n}\delta_{n,2p+1} \right) \epsilon, \\
(b) &\approx \left( 0, \frac{1}{4} - \frac{0.33}{n}\delta_{n,2p} - \frac{0.28}{n}\delta_{n,2p+1}, \frac{0.94}{n}\delta_{n,2p+1}, \frac{1}{4} - \frac{0.17}{n}\delta_{n,2p} + \frac{0.12}{n}\delta_{n,2p+1} \right) \epsilon.
\end{aligned} \tag{30}$$

The first QCP describes the transition to the axial nematic order. The second QCP as  $n \rightarrow \infty$  possesses an  $O(4)$  symmetry, which, however, gets lifted once the  $1/n$  corrections are accounted for. Even though as  $n \rightarrow \infty$  such QCP controls transition to either nematic or axionic insulating phases depending on whether  $g_2 > g_4$  or  $g_4 > g_2$  respectively, when the  $1/n$  corrections are taken into account it describes a continuous QPT to the axionic insulating phase. The QCP (a) always describes continuous transition to the axial nematic phase. The actual nature of the broken symmetry phase can be identified unambiguously when we examine the flow of various source terms along with the flow of local four-fermion coupling constants, as described in the following section.

## V. FLOW OF SOURCE TERMS

In the presence of all possible symmetry allowed source terms (in the particle-hole or excitonic channels) or fermionic bilinears the effective single particle Hamiltonian reads as

$$\begin{aligned}
H_{source}^{p-h} &= \int d^3x \left[ \Delta_0 \Psi^\dagger \Psi + \sum_{j=1}^2 [\Delta_1 (\Psi^\dagger \gamma_j \Psi + \Psi^\dagger \Gamma_{j5} \Psi) + \Delta_2 \Psi^\dagger \Gamma_{0j} \Psi + \Delta_3 \Psi^\dagger \Gamma_{j3} \Psi] + \Delta_4 [\Psi^\dagger \gamma_0 \Psi + \Psi^\dagger \Gamma_{50} \Psi] \right. \\
&\quad \left. + \Delta_5 [\Psi^\dagger \gamma_3 \Psi + \Psi^\dagger \Gamma_{35} \Psi] + \Delta_6 \Psi^\dagger \gamma_5 \Psi + \Delta_7 \Psi^\dagger \Gamma_{03} \Psi + \Delta_8 \Psi^\dagger \Gamma_{12} \Psi \right].
\end{aligned} \tag{31}$$

To the leading order, the RG flow equations of the source terms are given by

$$\begin{aligned}
\bar{\beta}_{\Delta_0} &= \frac{1}{4} [-3\lambda_0 + 2(\lambda_2 + \lambda_3 + \lambda_4)] f_2(n), \quad \bar{\beta}_{\Delta_1} = 0, \quad \bar{\beta}_{\Delta_2} = \left[ 2\lambda_2 + \lambda_4 - \frac{\lambda_0}{2} \right] f_1(n), \quad \bar{\beta}_{\Delta_3} = \left[ 2\lambda_3 - \lambda_4 - \frac{\lambda_0}{2} \right] f_1(n), \\
\bar{\beta}_{\Delta_4} &= \left[ 2\lambda_4 + \lambda_2 - \lambda_3 - \frac{\lambda_0}{2} \right] \times \left[ f_1(n) + \frac{1}{2} f_2(n) \right], \quad \bar{\beta}_{\Delta_5} = \left[ -\frac{\lambda_0}{2} - \lambda_2 + \lambda_3 \right] \times \left[ f_1(n) - \frac{1}{2} f_2(n) \right], \\
\bar{\beta}_{\Delta_6} &= [\lambda_0 + 2\lambda_2 + 2\lambda_3 - 2\lambda_4] \frac{f_2(n)}{4}, \quad \bar{\beta}_{\Delta_7} = [-\lambda_0 + 2\lambda_2 + 2\lambda_3 + 2\lambda_4] \frac{f_2(n)}{4}, \quad \bar{\beta}_{\Delta_8} = [-\lambda_0 + 2\lambda_2 + 2\lambda_3 - 2\lambda_4] \frac{f_2(n)}{4},
\end{aligned} \tag{32}$$

where  $\bar{\beta}_{\Delta_j} = \Delta_j^{-1} \beta_{\Delta_j} - 1$ .

We also examine the flow of the source terms associated with local (momentum independent) pairings. All together there are six local pairings and the corresponding Hamiltonian reads as

$$H_{source}^{p-p} = \int d^3x \left[ \Delta_1^{pp} \Psi \Gamma_{13} \Psi + \Delta_2^{pp} \Psi \Gamma_{02} \Psi + \Delta_3^{pp} \Psi \Gamma_{33} \Psi + \Delta_4^{pp} \Psi \Gamma_{05} \Psi + \Delta_5^{pp} \Psi \Gamma_{11} \Psi + \Delta_6^{pp} \Psi \Gamma_{25} \Psi \right]. \tag{33}$$

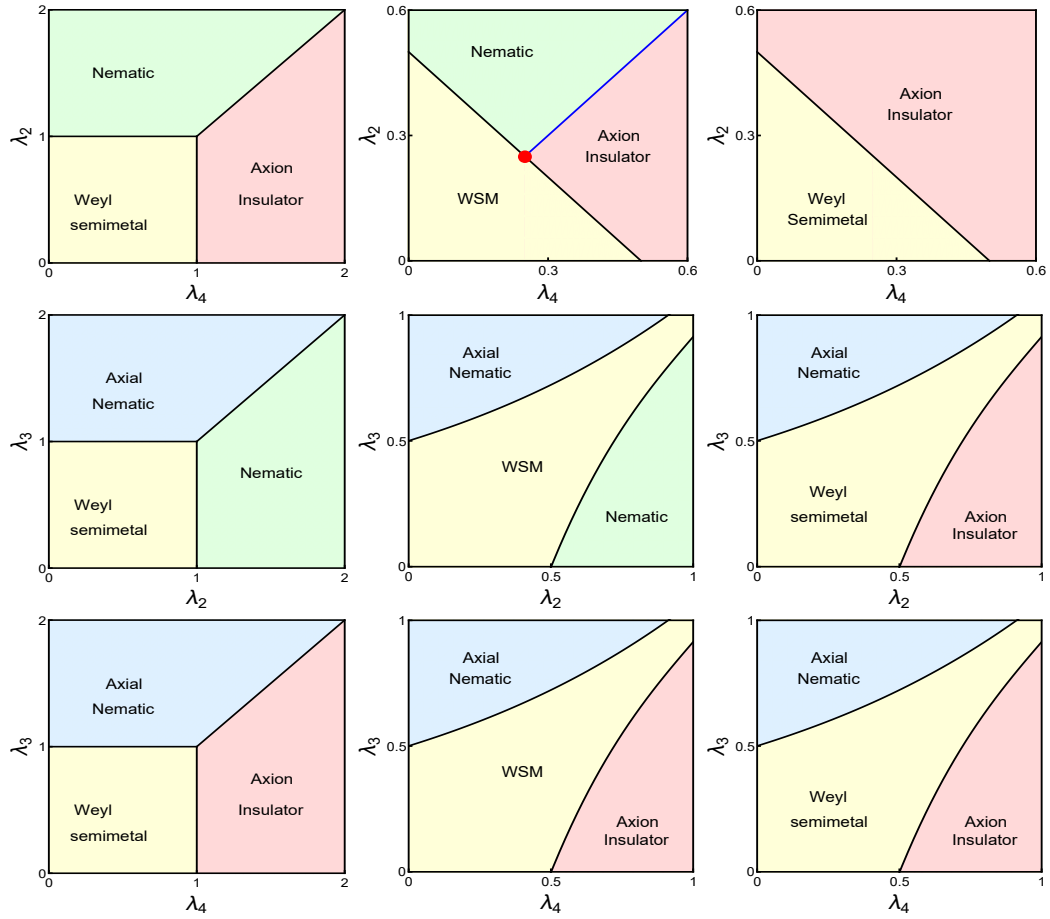

Figure 1: Evolution of various cuts of the phase diagram of interacting general WSMs obtained from (a) mean-field theory (left column), (b) from RG calculation in  $n \rightarrow \infty$  limit (center column), (c) from RG calculation after accounting for  $1/n$  corrections (but still  $n$  is large). Here red dot corresponds to a  $O(4)$  symmetric quantum critical point, and  $O(4)$  symmetry is spontaneously broken along the blue line. The Weyl semimetal-broken symmetry phase transitions are always continuous.

Note that all six  $4 \times 4$  matrices appearing in  $H_{source}^{p-p}$  are purely imaginary, as required due to *Pauli exclusion principle*. The RG flow equation for these source terms read as

$$\begin{aligned} \bar{\beta}_{\Delta_1^{pp}} &= \left[ \frac{\lambda_0}{2} - \lambda_2 - \lambda_3 \right] \times \left[ f_1(n) + (-1)^n \frac{1}{2} f_2(n) \right] = \bar{\beta}_{\Delta_2^{pp}}, \quad \bar{\beta}_{\Delta_3^{pp}} = \left[ \frac{\lambda_0}{2} - \lambda_4 \right] \times f_1(n) = \bar{\beta}_{\Delta_4^{pp}}, \\ \bar{\beta}_{\Delta_5^{pp}} &= (-1)^n \left[ \frac{\lambda_0}{2} - \lambda_2 + \lambda_3 - \lambda_4 \right] \times \frac{1}{2} f_2(n), \quad \bar{\beta}_{\Delta_6^{pp}} = (-1)^n \left[ -\frac{\lambda_0}{2} - \lambda_2 + \lambda_3 - \lambda_4 \right] \times \frac{1}{2} f_2(n), \end{aligned} \quad (34)$$

where  $n$  is an integer. Note that even-odd effect only appears on the RG flow of source terms in the particle-particle channels.

The scheme of identifying the broken symmetry phase is the following. We simultaneously run the RG flow for four-fermion coupling constants [see Eq. (29)] and source terms [see Eq. (32)]. For weak enough interactions all four-fermion couplings flow back to the trivial fixed point and none of the source term diverges. On the other hand, beyond critical strength of interaction at least one coupling constant diverges, which corresponds to the relevant direction of the quantum-critical point describing the actual transition, and the RG flow of at least one of the source terms blows up. The broken symmetry phase corresponds to the source term that diverges fastest among all possible source terms. Following this strategy we find the phase diagrams in various coupling constant spaces, reported in the main part of the paper. We display the evolution of phase diagrams in various coupling constant spaces in Fig. 1, obtained (a) within the mean-field approximation (left column), (b) from RG calculation to the leading order in  $\epsilon = 2/n$  upon setting  $n \rightarrow \infty$  (center column), (c) from RG calculation after accounting for  $1/n$  corrections (right column). It is

evident from this comparative study that both nature of the phase diagram and of broken symmetry phases at strong coupling change dramatically once the fluctuation effects are accounted for systematically. The phase diagrams from the right column of Fig. 1 have been summarized in Fig. 2 of the main part of the paper.

## VI. SOLUTION OF THE GAP EQUATION IN AXIONIC INSULATOR PHASE IN A GENERAL WSM

One of the direct consequences of non-Gaussian criticality is the the absence of *logarithmic correction* in various physical observables inside the ordered phases. For the sake of simplicity we here focus on the axion insulator (AI) phase, and for concreteness we consider the scaling of spectral gap which one can obtain from the mean-field gap equation. The mean-field free energy density in the presence AI order ( $\Delta_{AI}$ ) reads as

$$F = \frac{\Delta_{AI}^2}{2g_4} - 2 \int \frac{d^3\mathbf{k}}{(2\pi)^3} \sqrt{\alpha_n^2 k_{\perp}^{2n} + v^2 k_z^2 + \Delta_{AI}^2}. \quad (35)$$

While arriving at the last expression we have used the fact that sufficiently strong interaction denoted by  $g_5$  [see Eq. (3) of main text] supports AI phase. Minimizing the free-energy with respect to  $\Delta_{AI}$  we arrive at the mean-field gap equation

$$\frac{1}{2g_4} - \int \frac{d^3\mathbf{k}}{(2\pi)^3} \frac{1}{\sqrt{\alpha_n^2 k_{\perp}^{2n} + v^2 k_z^2 + \Delta_{AI}^2}} = 0. \quad (36)$$

After introducing a new set of coordinates

$$\alpha_n k_{\perp}^n = \rho \cos \theta, \quad v k_z = \rho \sin \theta, \quad \text{with } 0 \leq \rho \leq E_c, \quad -\frac{\pi}{2} \leq \theta \leq \frac{\pi}{2}, \quad (37)$$

where  $E_c$  is the ultraviolet energy cut-off for Weyl fermion, and defining a set of dimensionless variables as

$$\frac{\rho}{E_c} = x, \quad \frac{\Delta_{AI}}{E_c} = m, \quad \lambda_4 = g_4 \frac{2}{n} \frac{E_c^{2/n}}{v \alpha_n^{2/n}} \frac{1}{(2\pi)^3}, \quad (38)$$

we can write down the above gap equation compactly as

$$\frac{1}{\lambda_4} = \int_{-\pi/2}^{\pi/2} \cos^{\frac{2}{n}-1} \theta d\theta \int_0^1 \frac{x^{2/n}}{\sqrt{x^2 + m^2}} dx. \quad (39)$$

The above gap equation supports a non-trivial solution of the order parameter ( $m$ ) only when interaction  $\lambda_5$  is stronger than a critical value  $\lambda_5^*$ , given by

$$\frac{1}{\lambda_4} = \int_{-\pi/2}^{\pi/2} \cos^{\frac{2}{n}-1} \theta d\theta \int_0^1 x^{\frac{2}{n}-1} dx. \quad (40)$$

The universal scaling of the order parameter  $m$  is then obtained from the following equation [obtained by subtracting Eq. (40) from Eq. (39)]

$$\frac{1}{\lambda_4} - \frac{1}{\lambda_4^*} = \int_{-\pi/2}^{\pi/2} \cos^{\frac{2}{n}-1} \theta d\theta \int_0^1 x^{2/n} \left[ \frac{1}{\sqrt{x^2 + m^2}} - \frac{1}{x} \right]. \quad (41)$$

Let us now define a quantity  $\delta = \lambda_4^{-1} - (\lambda_4^*)^{-1}$  that measures the distance from the the critical point located at  $\lambda_4 = \lambda_4^*$ . For subcritical interaction  $\lambda_4 < \lambda_4^*$ ,  $\delta > 0$ , while for the interaction stronger than the critical value,  $\lambda_4 > \lambda_4^*$ ,  $\delta < 0$ . The universal scaling of the spectral gap in the AI phase is then determined by

$$\delta = -\frac{\sqrt{\pi} \Gamma\left(\frac{1}{n}\right)}{\Gamma\left(\frac{1}{n} + \frac{1}{2}\right)} \left[ \frac{n}{2} - {}_2F_1\left(\frac{1}{2}, \frac{1}{n} + \frac{1}{2}, \frac{1}{n} + \frac{3}{2}, -\frac{1}{m^2}\right) \right], \quad (42)$$

where  ${}_2F_1$  is the hypergeometric function. The right hand side of the above equation is a negative definite function of  $n$  and  $m$ , suggesting that non-trivial solution of the AI order parameter  $m$  can only be found for  $\delta < 0$  or  $\lambda_5 > \lambda_5^*$ .

Explicitly for  $n = 1$  and  $n = 2$  Eq. (42) respectively reduces to

$$\delta = -\frac{1}{2} \left[ 1 - \sqrt{1 + m^2} + m^2 \operatorname{csch}^{-1}(m) \right], \quad \delta = -\frac{\pi}{2} \left[ 1 + m - \sqrt{1 + m^2} \right] \quad (43)$$

Thus scaling of spectral gap in a simple WSM ( $n = 1$ ) possesses logarithmic corrections stemming from the mean-field nature of the QPT from the WSM to AI phase, captured by CLE  $\nu = 1/2$ . On the other hand, the scaling of the same quantity in a general WSM with  $n > 1$  (see the above equation for  $n = 2$ ) is devoid of any logarithmic correction, which is a direct manifestation of non-Gaussian criticality, captured by CLE  $\nu = n/2 > 1/2$  for  $n > 1$ .

## VII. FREE-ENERGY AT WSM-BI QCP IN THE PRESENCE OF SHORT-RANGE INTERACTION

This section is devoted to demonstrate the derivation of the free-energy [see Eq. (6) of main text] at the WSM-BI QCP in the presence of short-range interaction. This methodology can easily be generalized to arrive at the expression of the free-energy shown in Eq. (35). The partition function for critical excitations in the presence of local interaction  $\tilde{g}_3$  reads as

$$\begin{aligned} \mathcal{Z} &= \int \mathcal{D}\psi \mathcal{D}\psi^\dagger \exp \left[ - \int dt d^3\mathbf{x} \left\{ \psi^\dagger [-i\partial_t + H_n(\mathbf{k} \rightarrow -i\nabla)] \psi + \frac{\tilde{g}_3}{2} (\psi^\dagger \sigma_3 \psi)^2 \right\} \right], \\ &= \int \mathcal{D}\psi \mathcal{D}\psi^\dagger \mathcal{D}\lambda \exp \left[ - \int dt d^3\mathbf{x} \left\{ \psi^\dagger [-i\partial_t + H_n(\mathbf{k} \rightarrow -i\nabla)] \psi + \Sigma \psi^\dagger \sigma_3 \psi - \frac{\Sigma^2}{2\tilde{g}_3} \right\} \right]. \end{aligned} \quad (44)$$

To arrive at the final expression for the partition function we have decoupled the four-fermion interaction (proportional to  $\tilde{g}_3$ ) by the Hubbard-Stratonovich field  $\Sigma$  using an exact Gaussian integral, and  $H_n$  is the Hamiltonian shown in Eq. (1) of the main text. Now  $\mathcal{Z}$  is a quadratic function of fermionic field and we can readily integrate out fermion, yielding the following effective action

$$S_{eff} = \frac{1}{2\tilde{g}_3} \int_0^\beta dt \int d^3\mathbf{x} \Sigma^2(t, \mathbf{x}) - \operatorname{Tr} \ln [i\omega + \alpha_n k_\perp^n [\sigma_1 \cos(n\phi_{\mathbf{k}}) + \sigma_2 \sin(n\phi_{\mathbf{k}})] + \sigma_3 (Bk_z^2 + \Delta) + \sigma_3 \Sigma]. \quad (45)$$

We now restrict ourselves to the saddle point, so that fluctuations of the Hubbard-Stratonovich field  $\Sigma$  can be neglected. The expression of the mean-field free-energy density at  $T = 0$  reads as

$$F = \frac{\Sigma^2}{2\tilde{g}_3} - \int_{-\infty}^{\infty} \frac{d\omega}{2\pi} \int \frac{d^3\mathbf{k}}{(2\pi)^3} \ln [\omega^2 + \alpha_n^2 k_\perp^{2n} + (Bk_z^2 + \Delta + \Sigma)^2] \quad (46)$$

Notice that the integral over the Matsubara frequency is divergent. To eliminate such divergence we define a modified free-energy as

$$F + \int_{-\infty}^{\infty} \frac{d\omega}{2\pi} \int \frac{d^3\mathbf{k}}{(2\pi)^3} \ln \omega^2 \rightarrow F. \quad (47)$$

The regulated free-energy density after performing the integral over the Matsubara frequency reads as

$$F = \frac{\Sigma^2}{2\tilde{g}_3} - \int \frac{d^3\mathbf{k}}{(2\pi)^3} \sqrt{\alpha_n^2 k_\perp^{2n} + (Bk_z^2 + \Delta + \Sigma)^2}, \quad (48)$$

which is identical to Eq. (6) of the main text. To proceed with the calculation next we define a set of new variables

$$\alpha_n k_\perp^n = \eta \sin \theta, \quad Bk_z^2 = \eta \cos \theta, \quad \text{where } 0 < \eta < E_\Lambda, 0 \leq \theta \leq \pi/2, \quad (49)$$

where  $E_\Lambda$  is the ultraviolet energy cut-off for the critical excitation. After some tedious but otherwise straightforward algebra, we arrive at the compact expression for the dimensionless free-energy density

$$f = \frac{\rho^2}{2\lambda} - \int_0^1 dx x^{\frac{4-n}{2n}} \int_0^1 dy y^{-1/2} (1-y^2)^{-1+\frac{1}{n}} \sqrt{x^2(1-y^2) + (xy + m + \rho)^2}. \quad (50)$$

Various dimensionless quantities appearing in the final expression are defined as

$$f = \frac{F}{a_n E_\Lambda^{\frac{4+3n}{2n}}}, \quad \lambda = \tilde{g}_3 a_n E_\Lambda^{\frac{4-n}{2n}}, \quad \rho = \frac{\Sigma}{E_\Lambda}, \quad m = \frac{\Delta}{E_c}, \quad x = \frac{\eta}{E_\Lambda}, \quad y = \cos \theta. \quad (51)$$
